# Supplementary material for: Decomposable Non-Smooth Convex Optimization with Nearly-Linear Gradient Oracle Complexity
Source: arXiv:2208.03811 source file (2022-08-07)
Supplement: Supplementary file 1 [file our-appendix.tex]

\appendix
Our appendix is organized as follows. \cref{sec:AppendixPrelims} lays out all the preliminaries for the proof details of the paper; \cref{subsec:PotentialFns} shows the analysis of the algorithm; \cref{sec:init} shows the initialization, and \cref{sec:decompSFM} contains details about submodular function minimization as it pertains to our problem. 

\section{Preliminaries}\label{sec:AppendixPrelims}
\input{factsFromFoundations}

\input{analysis}

\input{initialization}

\input{decomp_SFM}
